# Supplementary material for: Every Camera Effect, Every Time, All at Once: 4D Gaussian Ray Tracing for Physics-based Camera Effect Data Generation
Source: arXiv:2509.10759 source file (2026-10-31)
Supplement: Supplementary file 1 [file supp_llm_experiment.tex]

\section{LLM Evaluation}

To evaluate whether large language models (LLMs) can achieve the same level of understanding when processing visual data with camera effects compared to normal (pinhole) images, we designed an experiment based on Multiple-Choice Prompting (MCP). The total accuracies are reported in table~\ref{tab:camera_effect_expriment_table}. This approach quantifies the image understanding capabilities of LLMs and directly compares performance differences between normal and camera effect images under identical scene conditions. We evaluated two LLMs: gemini-2.5-pro and gemini-2.5-flash, via Vertex AI (Google Cloud). See the Gemini 2.5 Technical Report~\cite{gemini25_report} and the official model card~\cite{gemini25_pro_card} for details. Section~\ref{sec:image_datasets} introduces the image datasets used in our evaluation, while Section~\ref{sec:camera_parameter_estimation} details our evaluation methodology and experimental design, and concludes with a summary of the observed performance trends across different camera effects. This includes highlighting cases where the presence of specific effects consistently degraded LLM accuracy, as well as rare instances where certain distortions appeared to provide unintended cues for parameter estimation.

\subsection{Image Datasets}
\label{sec:image_datasets}
We utilized three publicly available camera effect datasets: \textbf{FIORD}~\cite{gunes2025fiordfisheyeindooroutdoordataset} (fisheye), \textbf{Rolling-Shutter Visual-Inertial Odometry Dataset}~\cite{8968539} (rolling shutter), and \textbf{DFD dataset}~\cite{carvalho2018deepdepthdefocusdefocus} (depth of field). These datasets contain both normal images and corresponding camera effect images, forming paired image data. Through this paired design, we ensure that comparison results reflect solely the influence of camera effects without interference from image content variations.

\subsection{Camera Parameter Estimation}
\label{sec:camera_parameter_estimation}

We hypothesize that LLMs struggle to infer camera parameters when images contain camera effects. We therefore convert ground-truth parameters into four-choice questions for two tasks—\textbf{Aperture} and \textbf{Focal length}—and evaluate under fisheye, rolling-shutter (RS), and depth-of-field (DoF) conditions (100 samples per setting).

\textbf{Fisheye.}
Both models show degraded accuracy across tasks. For \texttt{gemini-2.5-pro}, Aperture (F2.2) drops from 71\% (\emph{Normal}) to 42\% (\emph{Effect}, $-29\%$), and Focal Length (2.41mm) from 99\% to 86\% ($-13\%$).
For \texttt{gemini-2.5-flash}, Aperture (F2.2) remains at 0\% in both conditions ($0\%$ change), while Focal Length (2.41mm) decreases from 55\% to 47\% ($-8\%$).
These results indicate that fisheye distortion generally harms parameter recognition.

\textbf{Rolling Shutter.}
Aperture estimation is notably weak and below the 25\% chance level for both models: \texttt{gemini-2.5-pro} falls from 18\% to 12\% ($-6\%$) and \texttt{gemini-2.5-flash} from 5\% to 2\% ($-3\%$).
In contrast, focal-length estimation is stable or slightly improved: \texttt{gemini-2.5-pro} is nearly unchanged (Focal Length 4mm: 100\% $\to$ 99\%, $-1\%$), while \texttt{gemini-2.5-flash} shows a small gain (88\% $\to$ 93\%, $+5\%$), suggesting RS geometry can occasionally provide extra cues for focal length.

\textbf{Depth of Field.}
With shallow DoF (F2.8) versus F8.0, aperture estimation improves: \texttt{gemini-2.5-pro} increases from 9\% to 86\% ($+77\%$) and \texttt{gemini-2.5-flash} from 35\% to 39\% ($+4\%$).
The clear–blur contrast in shallow DoF probably helps in the determination of the aperture value.

Overall, camera effects generally reduce the accuracy for camera parameter questions, with several fisheye/RS settings at or below chance. Exceptions include focal-length estimation under RS and aperture estimation under DoF, where the effect may introduce cues that aid recognition.

\subsection{Prompt Templates and MCP Settings}
\label{sec:prompt}
\paragraph{Models.} \texttt{gemini-2.5-pro}, \texttt{gemini-2.5-flash}.
\paragraph{Protocol.} Options are shuffled per query; output must match \texttt{[A|B|C|D]}. Non-compliant outputs are counted as incorrect.

\paragraph{System prompt (shared).}
\begin{quote}
\textit{``\textbf{Role}: You are a highly experienced professional photographer with an extensive portfolio and deep knowledge of camera techniques, composition, and post-processing effects.
Your expertise allows you to discern subtle nuances in the characteristics of the image.''}
\end{quote}

\paragraph{Prompt template.} We replace [EFFECT] with {fisheye | rolling shutter | depth of field}.
\begin{quote}
\textit{``\textbf{[EFFECT] Image Analysis Task:}\\
\textbf{Question:}\\
Based on your visual analysis of that specific image's unique structure and lens characteristics, determine the specific camera parameters, and select the most fitting option as your answer.\\
\textbf{Options:}\\
A)...\\
B)...\\
C)...\\
D)...\\
\textbf{Answer:}\\
Please select at least one and only one option that is the most appropriate(e.g., A, B, C, D).\\
Only answer the option, no reasoning.''}
\end{quote}

\begin{table}[t]
\centering
\caption{We design 4-choice MCPs to evaluate Gemini-2.5 models on estimating camera parameters~\cite{fang2025camerabench} (aperture or focal length) under images with fisheye distortion, rolling shutter, and depth of field (DoF) effect. For fisheye and rolling shutter, we compare images with and without the effect (‘Effect’ vs. ‘Normal’). For DoF, we use F8.0 as ‘Normal’ and F2.8 as ‘Effect’. We report accuracy on both settings and measure the change from normal to effect images. Results show that fisheye and rolling shutter consistently degrade accuracy, while varying DoF significantly impacts parameter estimation.
}
\label{tab:camera_effect_expriment_table}
\footnotesize

\resizebox{0.8\textwidth}{!}{
\begin{tabular}{l l l c c c}
\toprule
\textbf{Camera Effect} & \textbf{Model} & \textbf{Task} & \textbf{Normal} & \textbf{Effect} & \textbf{Change} \\
\midrule
\multirow{4}{*}{Fisheye} 
& \multirow{2}{*}{gemini-2.5-pro}   & Aperture ($f$/2.2)          & 71\%  & 42\%  & $-29\%$ \\
&                                   & Focal Length (2.41mm)    & 99\%  & 86\%  & $-13\%$ \\
\cline{2-6}\addlinespace[1.8pt]
& \multirow{2}{*}{gemini-2.5-flash} & Aperture ($f$/2.2)          & 0\%   & 0\%   & $0\%$ \\
&                                   & Focal Length (2.41mm)    & 55\%  & 47\%  & $-8\%$ \\
\midrule
\multirow{4}{*}{Rolling Shutter} 
& \multirow{2}{*}{gemini-2.5-pro}   & Aperture ($f$/1.8)          & 18\%  & 12\%  & $-6\%$ \\
&                                   & Focal Length (4mm)       & 100\% & 99\%  & $-1\%$ \\
\cline{2-6}\addlinespace[1.8pt]
& \multirow{2}{*}{gemini-2.5-flash} & Aperture ($f$/1.8)          & 5\%   & 2\%   & $-3\%$ \\
&                                   & Focal Length (4mm)       & 88\%  & 93\%  & $+5\%$ \\
\midrule
\multirow{2}{*}{Depth of Field} 
& gemini-2.5-pro   & Aperture ($f$/8.0 / $f$/2.8) & 9\%   & 86\%  & $+77\%$ \\
& gemini-2.5-flash & Aperture ($f$/8.0 / $f$/2.8) & 35\%  & 39\%  & $+4\%$ \\
\bottomrule
\end{tabular}
}
\end{table}
